# Supplementary material for: Algorithm-agnostic low-rank approximation of operator monotone matrix functions
Source: arXiv:2311.14023 source file (2024-07-04)
Supplement: Supplementary file 1 [file appendix.tex]

\begin{appendices}
\section{Proofs of Theorem~\ref{theorem:krylov_generalization} and Theorem~\ref{theorem:main_results}}\label{appendix:krylov_generalization}
\begin{proof}[Proof of Theorem~\ref{theorem:krylov_generalization}]
The proofs are identical to the proof of \cite[Lemma 9]{MM15}, and are included for completeness.
\proofpart{Proof of Property 1}{}
When $\gamma = \varepsilon$, if $m = 0$ or $x^* = \infty$ then the statement trivially holds. For $\gamma = \min\{1,\frac{g(\lambda_{k})-g(\lambda_{k+1})}{g(\lambda_{k+1})}\}$ then $m = k$. Henceforth, assume $m \geq 1$ and $x^* < \infty$. By Lemma~\ref{lemma:structural} we know
\begin{align}\label{eq:inequalities}
    \begin{split}
    &\|p_1(\bm{A}) - \bm{Y}_1 \bm{Y}_1^Tp_1(\bm{A})\|_F^2 \leq (1+\bm{\Omega}_2\bm{\Omega}_1^{-1}\|_2^2) \|p_1(\bm{\bm{A}})-p_1(\bm{\bm{A}})_k\|_F^2 \leq \\
    &(1+\bm{\Omega}_2\bm{\Omega}_1^{-1}\|_2^2) \sum\limits_{i=k+1}^n p_1(\lambda_i)^2 \leq n(1+\bm{\Omega}_2\bm{\Omega}_1^{-1}\|_2^2) \delta^{(q,\gamma)} g(\lambda_{k+1})^2 = \varepsilon g(\lambda_{k+1})^2.
    \end{split}
\end{align}
Define $\bm{C} = \bm{Y}_1^T \bm{U}$ and $c_i = \|\bm{C}_{i,:}\|_2 $. Note that $c_i \in [0,1]$. Hence, for $\ell \leq m$ we have
\begin{align}\label{eq:inequalities2}
    \begin{split}
    &\|p_1(\bm{A}) - \bm{Y}_1 \bm{Y}_1^Tp_1(\bm{A})\|_F^2 = \|p_1(\bm{\Sigma})\|_F^2 - \|\bm{C}p_1(\bm{\Sigma})\|_F^2 = \\
    &\sum\limits_{i=1}^n(1-c_i^2) p_1(\lambda_i)^2 \geq \sum\limits_{i=1}^{\ell}(1-c_i^2)p_1(\lambda_i)^2 \geq \\
    & \sum\limits_{i=1}^{\ell}(1-c_i^2)g(\sigma_i)^2 = \|g(\bm{A})_{\ell}\|_F^2 - \|\bm{Y}_1\bm{Y}_1^T g(\bm{A})_{\ell}\|_F^2 =\\
    &\|g(\bm{A}) - \bm{Y}_1\bm{Y}_1^Tg(\bm{A})_{\ell}\|_F^2 - \|g(\bm{A}) - g(\bm{A})_{\ell}\|_F^2,
    \end{split}
\end{align}
where we used that $g$ is increasing so that the singular values of the best rank $k$ approximation of $g(\bm{A})$ are $g(\lambda_i)$ for $i = 1,\ldots,k$. Since $\bm{Y}_1\bm{Y}_1^T g(\bm{A})_{\ell}$ is a rank $\ell$ approximation whose range is contained in $\bm{Q}$ and by Lemma~\ref{lemma:constrained_best_low_rank_approximation} $\bm{Q}_{:,1:\ell} \bm{Q}_{:,1:\ell}g(\bm{A})$ is the best rank $\ell$ approximation whose range is contained in $\bm{Q}$ we have
\begin{equation}\label{eq:best_rank_k_in_Q}
    \|g(\bm{A}) - \bm{Y}_1\bm{Y}_1^Tg(\bm{A})_{\ell}\|_F^2 \geq \|g(\bm{A}) - \bm{Q}_{:,1:\ell}\bm{Q}_{:,1:\ell}^Tg(\bm{A})\|_F^2.
\end{equation}
Combining the inequalities \eqref{eq:inequalities}-\eqref{eq:best_rank_k_in_Q} yields Property 1. 

\proofpart{Proof of Property 2}{}
Note that by Pythagoras theorem, Property 1 immediately implies Property 2 for $\ell \leq m$. Hence, it suffices to show the result for $\ell > m$ if $m < k$. Note that if $w = 0$ we have $m = k$. Thus, we henceforth assume that $w \geq 1$.

Partition $\bm{A}$ as 
\begin{equation*}
    \bm{A} = \begin{bmatrix} \bm{U}_1 & \bm{U}_2^{(1)} & \bm{U}_2^{(2)} \end{bmatrix} \begin{bmatrix} \bm{\Lambda}_1 & & \\ & \bm{\Lambda}_2^{(1)} & \\ & & \bm{\Lambda}_2^{(2)} \end{bmatrix} \begin{bmatrix} \bm{V}_1^T \\ \bm{V}_2^{(1)T} \\ \bm{V}_2^{(2)T}
    \end{bmatrix},
\end{equation*}
where $\bm{\Sigma}_2^{(1)} \in \mathbb{R}^{w \times w}$ contains all singular values so that $\frac{g(\lambda_k)}{1+\gamma} \leq g(\lambda_i) < g(\lambda_k)$. Define
\begin{equation*}
    \bm{B}^{(1)} = \bm{U}_2^{(1)} p_2(\bm{\Sigma}_2^{(1)}) \bm{V}_2^{(1)T}, \quad \bm{B}^{(2)} = p_2(\bm{A}) - \bm{B}^{(1)}.
\end{equation*}
Let $\bm{Y}^{(1)}_2$ and $\bm{Y}^{(2)}_2$ be orthonormal bases for $\range(\bm{B}^{(1)} \bm{\Omega})$ and $\range(\bm{B}^{(2)} \bm{\Omega})$ respectively. We know that $\range(\bm{B}^{(1)})$ and $\range(\bm{B}^{(2)})$ are orthogonal subspaces. Consequently, $\begin{bmatrix} \bm{Y}^{(1)} & \bm{Y}^{(2)} \end{bmatrix}$ is an orthonormal basis. Furthermore, since $p_2(\bm{A})\bm{\Omega} = \bm{B}^{(1)} \bm{\Omega} + \bm{B}^{(2)} \bm{\Omega}$ we have that for any $\bm{x} \in \range(p_2(\bm{A}) \bm{\Omega})$ there exists $\bm{x}^{(1)} \in \range(\bm{Y}^{(1)})$ and $\bm{x}^{(2)} \in \range(\bm{Y}^{(2)})$ such that $\bm{x} = \bm{x}^{(1)} + \bm{x}^{(2)}$. Hence, for any $\bm{x}\in \range(p_2(\bm{A})\bm{\Omega})$ we have
\begin{equation}\label{eq:decomposition}
    \|\bm{x}^Tg(\bm{A})\|_2^2 =  \|\bm{x}^{(1)T}g(\bm{A})\|_2^2 +  \|\bm{x}^{(2)T}g(\bm{A})\|_2^2.
\end{equation}
We will bound each term in \eqref{eq:decomposition} separately. Note that $\bm{x}^{(1)} = \bm{U}_2^{(1)} \bm{z}^{(1)}$ for some $\bm{z}^{(1)}$. Hence,
\begin{equation}\label{eq:first_inequality}
    \|\bm{x}^{(1)T}g(\bm{A})\|_2^2 = \bm{z}^{(1)T} \bm{\Sigma}_2^{(1)2} \bm{z}^{(1)} \geq \frac{1}{(1+\varepsilon)^2} g(\lambda_k)^2\|\bm{x}^{(1)}\|_2^2.
\end{equation}
Furthermore,
\begin{align*}
    &\|\bm{B}^{(2)}-\bm{Y}_2^{(2)}\bm{Y}_2^{(2)T}\bm{B}^{(2)}\|_F^2 \leq (1+\|\bm{\Omega}_2\bm{\Omega}_1^{-1}\|_2^2)\sum\limits_{i=k+w+1}^n p_2(\lambda_i)^2 \leq \\
    &\frac{\varepsilon g(\lambda_k)^2}{(1+\varepsilon)^2}.
\end{align*}
Furthermore, using the same technique as in Lemma~\ref{lemma:property1} and using $g(\bm{A})_k = \bm{B}^{(1)}_k$ we can show 
\begin{equation}\label{eq:Y_outer_good}
    \|g(\bm{A})_k - \bm{Y}_2^{(2)}\bm{Y}_2^{(2)T}g(\bm{A})_k\|_F^2 \leq \frac{\varepsilon g(\lambda_k)^2}{(1+\varepsilon)^2}.
\end{equation}
Hence, following \cite[Equation (11)]{MM15} we have for any $\bm{x}^{(2)} \in \range(\bm{Y}^{(2)})$ that
\begin{equation}\label{eq:second_inequality}
    (1-\frac{\varepsilon}{(1+\varepsilon)^2})g(\lambda_k)^2\|\bm{x}^{(2)}\|_2^2 \leq \|\bm{x}^{(2)T}g(\bm{A})\|_2^2.
\end{equation}
Combining \eqref{eq:first_inequality} and \eqref{eq:second_inequality} with \eqref{eq:decomposition} we get for any $\bm{x} \in \range(p_2(\bm{A})\bm{\Omega})$ with unit norm we have
\begin{equation}\label{eq:large_innerprod}
    \|\bm{x}^{T}g(\bm{A})\|_2^2 \geq \min\left\{\frac{1}{(1+\varepsilon)^2}, 1-\frac{\varepsilon}{(1+\varepsilon)^2}\right\}g(\lambda_k)^2 = \frac{g(\lambda_k)^2}{(1+\varepsilon)^2}.
\end{equation}
Hence, since $\range(\bm{Y}_2) \subseteq \range(\bm{Q})$\footnote{\David{If $\bm{P}_1$ projects onto a subspace of the range of projector $\bm{P}_2$, then $\sigma_i(\bm{P}_1 \bm{A}) = \sigma_i(\bm{P}_1 \bm{P}_2 \bm{A}) \leq \|\bm{P}_1\|_2 \sigma_i(\bm{P}_2 \bm{A}) = \sigma_i(\bm{P}_2 \bm{A})$.}} we have for $\ell > m$
\begin{align*}
    &g(\lambda_{\ell})^2- \lambda_{\ell}\left(\bm{Q}\bm{Q}^T g(\bm{A})\right)^2 \leq (1+\varepsilon)^2 g(\lambda_{k+1})^2 - \lambda_{\ell}\left(\bm{Y}_1\bm{Y}_1^T g(\bm{A})\right)^2 = \\
    & ((1+\varepsilon)^2 - \frac{1}{(1+\varepsilon)^2}) g(\lambda_{k+1})^2 \leq 4\varepsilon g(\lambda_{k+1})^2,
\end{align*}
as required.

\proofpart{Proof of Property 3}{}
By Property 1 and Property 2 we already have 
\begin{equation}\label{eq:frob_inequality}
    \|g(\bm{A})-\bm{Q}_{:,1:\ell} \bm{Q}_{:,1:\ell}^T g(\bm{A})\|_F^2 \leq \|g(\bm{A})-g(\bm{A})_{\ell}\|_F^2 + \varepsilon g(\lambda_{k+1})^2 + 4(k-m) \varepsilon g(\lambda_{k+1})^2.
\end{equation}
Hence, if $k-m \leq w$ we are done. Henceforth, assume that $w < k-m$. Consequently, $\rank(\bm{B}^{(1)} \bm{\Omega}) = \rank(\bm{Y}^{(1)}_2) = w$. Thus, $\dim(\text{ker}(\bm{B}^{(1)} \bm{\Omega})) = k-w$. Hence, for any $\bm{x} \in \text{ker}(\bm{B}^{(1)} \bm{\Omega})$ we have
\begin{equation*}
    p_2(\bm{A}) \bm{\Omega}\bm{x} = \bm{B}^{(1)} \bm{\Omega} \bm{x} + \bm{B}^{(2)} \bm{\Omega} \bm{x} = \bm{B}^{(2)} \bm{\Omega} \bm{x}.
\end{equation*}
Hence, there is a $k-w$ dimensional subspace of $\range(p_2(\bm{A}) \bm{\Omega})$ that falls entirely in $\range(\bm{Y}_2^{(2)})$.

Note that if $\ell\leq m + w$ Property 1 and Property 2 already gives the desired inequality by \eqref{eq:frob_inequality}. Hence, now assume that $m + w < \ell \leq k$. Let $\mathcal{V} = \range(\bm{Y}_2^{(2)}) \cap \range(\bm{Y}_2)$ denote the $k-w$ dimensional subspace of $\range(\bm{Y}_2)$ entirely contained in $\range(\bm{Y}_2^{(2)})$. Note that
\begin{align*}
    &k-w = \dim\left(\mathcal{V} \right) = \dim\left(\left[\mathcal{V} \cap \range(\bm{Q}_{:,1:m})\right]  \oplus \left[\mathcal{V} \cap \range(\bm{Q}_{:,1:m})^{\bot}\right]\right) = \\
    & \dim\left(\mathcal{V} \cap \range(\bm{Q}_{:,1:m})\right)  +  \dim\left(\mathcal{V} \cap \range(\bm{Q}_{:,1:m})^{\bot}\right) \leq \\
    & m + \dim\left(\range(\bm{Y}_2^{(2)}) \cap \range(\bm{Q}_{:,1:m})^{\bot}\right).
\end{align*}
Hence, $0 < k-w-m \leq \dim\left(\range(\bm{Y}_2^{(2)}) \cap \range(\bm{Q}_{:,1:m})^{\bot}\right)$. Now, let $\bm{X}_1$ be an orthonormal basis for any $\min\{k-w-m,\ell-m\}$ dimensional subspace of $\range(\bm{Y}_2^{(2)}) \cap \range(\bm{Q}_{:,1:m})^{\bot}$. If $k-w-m < \ell-m$ then let $\bm{X}_2\in \mathbb{R}^{n \times (\ell - (k-w))}$ be an orthonormal basis for any $\ell - (k-w)$ dimensional subspace of the $w$ dimensional subspace $\range(\bm{Y}_2) \cap \range\left(\begin{bmatrix} \bm{Q}_{:,1:m} & \bm{X}_1 \end{bmatrix}\right)^{\bot}$. Otherwise, let $\bm{X}_2$ be empty. Define the orthonormal basis
\begin{equation*}
    \bar{\bm{Q}} = \begin{bmatrix} \bm{Q}_{:,1:m} & \bm{X}_1 & \bm{X}_2 \end{bmatrix} \in \mathbb{R}^{n \times \ell}
\end{equation*}
and partition
\begin{equation*}
    \bm{Y}_{2}^{(2)} = \begin{bmatrix} \bm{X}_1 & \bar{\bm{Y}} \end{bmatrix},
\end{equation*}
where $\bar{\bm{Y}} \in \mathbb{R}^{n \times (k-\min\{k-w-m,\ell-m\})}$. By \eqref{eq:Y_outer_good} we have
\begin{align*}
    &\frac{\varepsilon g(\lambda_k)^2}{(1+\varepsilon)^2} \geq \|g(\bm{A})_k - \bm{Y}_2^{(2)}\bm{Y}_2^{(2)T}g(\bm{A})_k\|_F^2 = \\
    &\|g(\bm{A})_k\|_F^2 - \|\bar{\bm{Y}}\bar{\bm{Y}}^T g(\bm{A})_k\|_F^2 - \|\bm{X}_1 \bm{X}_1^T g(\bm{A})_k\|_F^2 \geq \\
    &\sum\limits_{i=k-\min\{k-w-m,\ell-m\}}^k g(\sigma_i)^2 - \|\bm{X}_1 \bm{X}_1^T g(\bm{A})\|_F^2.
\end{align*}
Applying \eqref{eq:large_innerprod} to each column in $\bm{X}_2$ we have if $\bm{X}_2$ is non-empty
\begin{equation*}
    \|\bm{X}_2\bm{X}_2^T g(\bm{A})\|_F^2 \geq (\ell-w-k)\frac{g(\lambda_k)^2}{(1+\varepsilon)^2} \geq (\ell-w-k)\frac{g(\lambda_{k+1})^2}{(1+\varepsilon)^2}.
\end{equation*}

\end{proof}

\begin{proof}[Proof of Theorem~\ref{theorem:main_results}]
When $\gamma = \min\left\{1, \frac{g(\lambda_k)-g(\lambda_{k+1})}{g(\lambda_{k+1})}\right\}$ we have that $m = k$, so $(iii)$ immediately follows from Theorem~\ref{theorem:krylov_generalization} $(i)$. Furthermore, $(i)$ follows from \cite[Theorem 3.4]{gu_subspace}. Note that Theorem~\ref{theorem:krylov_generalization} $(i)$ implies that $\sum\limits_{i=1}^k(g(\lambda_i)^2 - \sigma_i(\bm{Q} \bm{Q}^T \bm{A})^2) \leq \varepsilon g(\lambda_{k+1})^2$ which implies $(ii)$. 

Now consider the case when $\gamma = \varepsilon$. Note that $(ii)$ is immediate from Theorem~\ref{theorem:krylov_generalization}, hence we focus on $(i)$ and $(iii)$. $(iii)$ follows from the fact that $(1+\varepsilon)\|g(\bm{A}) - g(\bm{A})_k\|_F^2 \geq w g(\sigma_{k})^2$. $(i)$ follows from 
\begin{align*}
    &\|(\bm{I}-\bm{Q}_{:,1:k}\bm{Q}_{:,1:k}^T)g(\bm{A})\|_2^2 \leq \|(\bm{I}-\bm{Q}_{:,1:m}\bm{Q}_{:,1:m}^T)g(\bm{A})\|_2^2 \leq \\
    &g(\lambda_{m+1})^2 + \varepsilon g(\lambda_{k+1})^2 \leq (1+2\varepsilon) g(\lambda_{k+1})^2,
\end{align*}
as required.
\end{proof}
\end{appendices}
